# Supplementary material for: Rates of convergence of the partial-wave expansion beyond Kato's cusp condition II: evaluations for the prefactors on the ground state of the helium atom
Source: arXiv:2107.01415 ancillary file (2021-07-03)
Supplement: Supplementary file 1 [file paper_II_si.pdf]

# *Supplementary Material for* Rates of convergence of the partial-wave expansion beyond the Kato's cusp condition II: evaluations for the prefactors

Cong Wang*

*Department of Chemistry, Michigan State University,*

*East Lansing, Michigan 48824, USA*

(Dated: July 2, 2021)

* wangcon9@msu.edu

## I. HIGHER-ORDER EXPRESSIONS OF THE FORMAL SOLUTION FOR THE FIRST-ORDER WAVEFUNCTION

$$\psi = \sum_{l=0}^{L} \psi_l P_l(\cos\theta_{12}) \tag{1}$$

To ensure the correctness of the next leading order expressions from Eq. (23) in Tables VI and VII in the main text, high-order expressions in the formal solution were used with the help of the software Mathematica [1]. Here we present the formulae

$$\psi = \sum_{n=0}^{\infty} r_{12}^n \phi_n \tag{2}$$

$$\phi_1 = \frac{1}{2}\Phi\left[1 - \frac{1}{3}s\eta^2 + \frac{1}{15}s^2\eta^4 - \left(\frac{1}{105}s^2 + \frac{1}{105}s^3\right)\eta^6 + \left(\frac{1}{315}s^2 + \frac{1}{315}s^3 + \frac{1}{945}s^4\right)\eta^8 - \left(\frac{1}{693}s^2 + \frac{1}{693}s^3 + \frac{2}{3465}s^4 + \frac{1}{10395}s^5\right)\eta^{10} + \cdots\right] \tag{3}$$

$$\phi_3 = \frac{1}{9}\Phi\left[\frac{1}{s} - \left(\frac{7}{8s} + \frac{2}{5}\right)\eta^2 + \left(\frac{1}{16s} + \frac{251}{560} + \frac{3s}{35}\right)\eta^4 - \left(\frac{3}{128s} + \frac{2171}{13440} + \frac{1577s}{13440} + \frac{4s^2}{315}\right)\eta^6 + \left(\frac{3}{256s} + \frac{8451}{98560} + \frac{10229s}{147840} + \frac{18229s^2}{887040} + \frac{s^3}{693}\right)\eta^8 + \cdots\right] \tag{4}$$

$$\phi_5 = \Phi\left[\frac{13}{360s^3} + \frac{4}{225s^2} - \left(\frac{3}{40s^3} + \frac{68}{1575s^2} + \frac{4}{525s}\right)\eta^2 + \left(\frac{5}{384s^3} + \frac{1417}{22400s^2} + \frac{3491}{201600s} + \frac{8}{4725}\right)\eta^4 \left(\frac{7}{960s^3} + \frac{63083}{1663200s^2} + \frac{8s}{31185} + \frac{493007}{19958400s} + \frac{80693}{19958400}\right)\eta^6 + \cdots\right] \tag{5}$$

$$\phi_7 = \Phi\left[\frac{37}{1680s^5} + \frac{653}{58800s^4} + \frac{8}{3675s^3} - \left(\frac{169}{2688s^5} + \frac{60373}{1411200s^4} + \frac{1503}{156800s^3} + \frac{32}{33075s^2}\right)\eta^2 + \left(\frac{7}{384s^5} + \frac{393109}{5174400s^4} + \frac{1156349}{46569600s^3} + \frac{191}{55440s^2} + \frac{16}{72765s}\right)\eta^4 + \cdots\right] \tag{6}$$

## II. ALTERNATIVE ASPECTS ON THE RATES OF CONVERGENCE OF PARTIAL-WAVE EXPANSION

If we reduce the upper limit of $m$ in Eq. (12) to $N-n+1$, $\chi$ will approach $r_{12}^{N+2}, (r_1 - r_2)^2 r_{12}^N, (r_1 - r_2)^4 r_{12}^{N-2}, \cdots$. Explicitly

$$\phi_1 = \frac{1}{2}\Phi, \qquad N=1 \qquad (7)$$

$$\phi_1 = \frac{1}{2}\Phi\left[1 - \frac{1}{3}s\eta^2\right], \phi_3 = \frac{1}{9s}\Phi, \qquad N=3 \qquad (8)$$

$$\phi_1 = \frac{1}{2}\Phi\left[1 - \frac{1}{3}s\eta^2 + \frac{1}{15}s^2\eta^4\right], \phi_3 = \frac{1}{9}\Phi\left[\frac{1}{s} - \left(\frac{7}{8s} + \frac{2}{5}\right)\eta^2\right], \phi_5 = \Phi\left[\frac{13}{360s^3} + \frac{4}{225s^2}\right], \qquad N=5 \qquad (9)$$

We shall refer this possibility as "minimum construction".

For the partial-wave expansion, there are three additional aspects: variational rates of convergence, expanded rates of convergence under the minimum construction, and variational rates of convergence under the minimum construction. We present the numerical results in Tables I-VI and Figures 1-6.

In general, fixing the amplitudes of germinal functions by the derivatives of the exact wavefunction at the coalescence region corresponds to local properties. The relaxations, especially at small $L$, mimick the global shape of the exact wavefunction. This aspect may provide an explanation for the effectiveness of combining fix amplitudes treatment and the Slater geminal function [2]. It may also imply that the sampling points [3] based on global measure, e.g. minimizing $H^2$ error [4], could be useful.

TABLE I. Numerical results of the variational PWE increments for the second-order-$1/Z$ expansion energies of the ground state of the helium atom. Eqs. (49) and (50) in the main text are used as the wavefunction in the Hylleraas functional [5] at $\omega = 30$. The atomic units are adopted.

| $L$ | $\lvert\tilde{E}_2(L) - \tilde{E}_2(L-1)\rvert$ | | |
|---|---|---|---|
| | $r_{12}\Phi_1 + \tilde{\chi}$ | $r_{12}\Phi_1 + r_{12}^3\Phi_3 + \tilde{\chi}$ | $r_{12}\Phi_1 + r_{12}^3\Phi_3 + r_{12}^5\Phi_5 + \tilde{\chi}$ |
| 0[a] | $1.282\times10^{-1}$ | $1.141\times10^{-1}$[b] | $6.089\times10^{-1}$[b] |
| 1 | $2.908\times10^{-2}$ | $2.696\times10^{-1}$ | $7.263\times10^{-1}$ |
| 2 | $3.299\times10^{-4}$ | $2.188\times10^{-3}$ | $4.009\times10^{-2}$ |
| 3 | $2.284\times10^{-5}$ | $1.234\times10^{-5}$ | $1.730\times10^{-4}$ |
| 4 | $3.173\times10^{-6}$ | $4.680\times10^{-7}$ | $5.710\times10^{-7}$ |
| 5 | $6.552\times10^{-7}$ | $3.848\times10^{-8}$ | $1.356\times10^{-8}$ |
| 6 | $1.756\times10^{-7}$ | $4.987\times10^{-9}$ | $7.348\times10^{-10}$ |
| 7 | $5.668\times10^{-8}$ | $8.791\times10^{-10}$ | $6.535\times10^{-11}$ |
| 8 | $2.103\times10^{-8}$ | $1.939\times10^{-10}$ | $8.165\times10^{-12}$ |
| 9 | $8.700\times10^{-9}$ | $5.077\times10^{-11}$ | $1.312\times10^{-12}$ |
| 10 | $3.926\times10^{-9}$ | $1.523\times10^{-11}$ | $2.560\times10^{-13}$ |
| 11 | $1.902\times10^{-9}$ | $5.102\times10^{-12}$ | $5.837\times10^{-14}$ |
| 12 | $9.777\times10^{-10}$ | $1.873\times10^{-12}$ | $1.512\times10^{-14}$ |
| 13 | $5.283\times10^{-10}$ | $7.429\times10^{-13}$ | $4.358\times10^{-15}$ |
| 14 | $2.979\times10^{-10}$ | $3.147\times10^{-13}$ | $1.377\times10^{-15}$ |
| 15 | $1.742\times10^{-10}$ | $1.411\times10^{-13}$ | $4.701\times10^{-16}$ |
| $\Delta E$[c] | $4.210 \times10^{-10}$ | $2.066 \times10^{-13}$ | $4.331 \times10^{-16}$ |

[a] The energy of $\lvert\tilde{E}_2(L)\rvert$, $L$=0.

[b] The energy is positive.

[c] The total energy at the largest $L$ subtracts the reference value, -0.15766 64294 69150 94105 66 a.u. [6]

TABLE II. Numerical results of the expanded PWE increments for the second-order-$1/Z$ expansion energies of the ground state of the helium atom under minimum construction. Eqs. (51) - (53) are used as the wavefunction at $\omega = 20$ in the Hylleraas functional [5]. The atomic units are adopted.

| $L$ | $\|E_2(L) - E_2(L-1)\|$ | | |
|---|---|---|---|
| | $r_{12}\Phi_1 + \chi$ | $r_{12}\Phi_1 + r_{12}^3\Phi_3 + \chi$ | $r_{12}\Phi_1 + r_{12}^3\Phi_3 + r_{12}^5\Phi_5 + \chi$ |
| $0^a$ | $1.179\times10^{-1}$ | $1.721\times10^{-1b}$ | $7.001\times10^{-1b}$ |
| 1 | $3.921\times10^{-2}$ | $3.267\times10^{-1}$ | $8.057\times10^{-1}$ |
| 2 | $4.821\times10^{-4}$ | $3.122\times10^{-3}$ | $5.182\times10^{-2}$ |
| 3 | $3.444\times10^{-5}$ | $1.941\times10^{-5}$ | $2.555\times10^{-4}$ |
| 4 | $4.858\times10^{-6}$ | $7.808\times10^{-7}$ | $9.336\times10^{-7}$ |
| 5 | $1.012\times10^{-7}$ | $6.664\times10^{-8}$ | $2.386\times10^{-8}$ |
| 6 | $2.726\times10^{-7}$ | $8.854\times10^{-9}$ | $1.363\times10^{-10}$ |
| 7 | $8.831\times10^{-8}$ | $1.588\times10^{-10}$ | $1.259\times10^{-11}$ |
| 8 | $3.286\times10^{-8}$ | $3.546\times10^{-10}$ | $1.616\times10^{-12}$ |
| 9 | $1.362\times10^{-9}$ | $9.371\times10^{-11}$ | $2.650\times10^{-12}$ |
| 10 | $6.159\times10^{-9}$ | $2.831\times10^{-11}$ | $5.250\times10^{-13}$ |
| 11 | $2.991\times10^{-9}$ | $9.536\times10^{-12}$ | $1.211\times10^{-14}$ |
| 12 | $1.541\times10^{-10}$ | $3.517\times10^{-12}$ | $3.165\times10^{-14}$ |
| 13 | $8.357\times10^{-10}$ | $1.401\times10^{-13}$ | $9.188\times10^{-15}$ |
| 14 | $4.731\times10^{-10}$ | $5.956\times10^{-13}$ | $2.916\times10^{-15}$ |
| 15 | $2.781\times10^{-10}$ | $2.681\times10^{-13}$ | $9.999\times10^{-16}$ |
| $\Delta E^c$ | $6.039\ \times10^{-10}$ | $3.843\ \times10^{-13}$ | $6.290\ \times10^{-16}$ |

[a] The energy of $|E_2(L)|$, $L$=0.

[b] The energy is positive.

[c] The total energy at the largest $L$ subtracts the reference value, -0.15766 64294 69150 94105 66 a.u. [6]

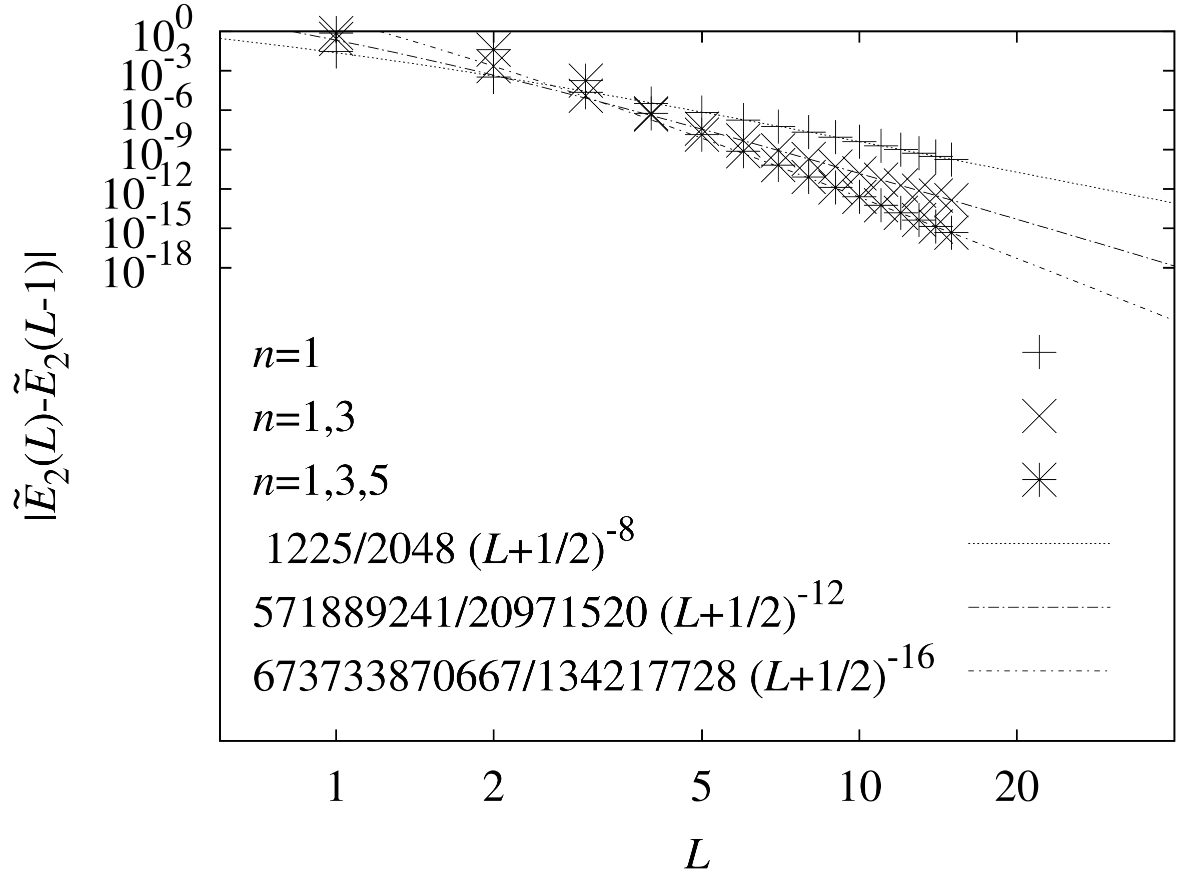


FIG. 1. $|\tilde{E}_2(L) - \tilde{E}_2(L-1)|$ via $L$ plot for the second-order $1/Z$ energy. The numerical data points are obtained from Table I. Atomic units are used in the figure.

## III. DETAILED DATA FOR "NUMERICAL RESULTS FOR THE $1/Z$ EXPANSIONS" AND "NUMERICAL RESULTS FOR THE PWE IN RITZ'S VARIATIONS"

The data including comparing with different orders of basis F ($\omega$=20 or 30) are presented in Tables VII - XIV.

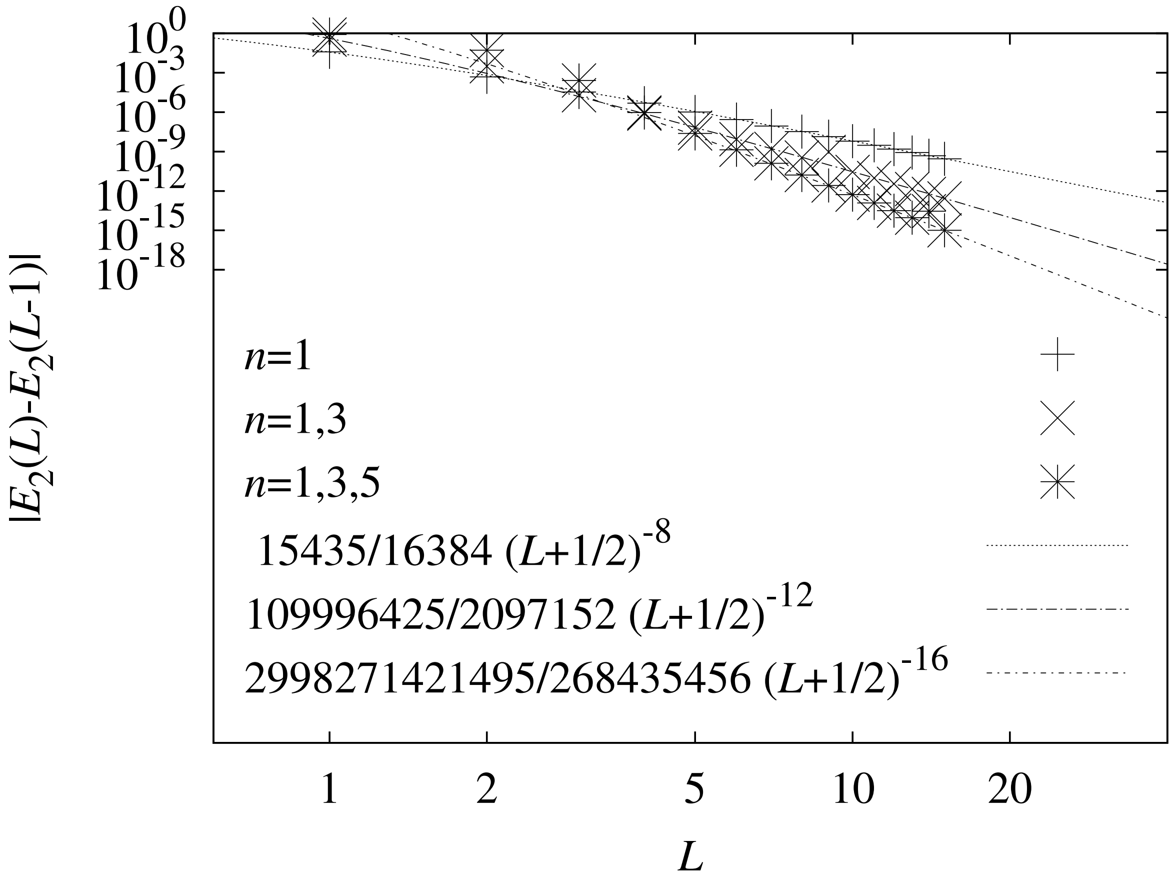


FIG. 2. $|E_2(L)-E_2(L-1)|$ via $L$ plot for the second-order $1/Z$ energy under minimum construction of geminal functions. The numerical data points are obtained from Table II. Atomic units are used in the figure.

---


[1] Wolfram Research, Inc., "Mathematica, Version 12.3.1," Champaign, IL, 2021.

[2] C. Hättig, W. Klopper, A. Köhn, and D. P. Tew, Chem. Rev. **112**, 4 (2012).

[3] H. Nakatsuji, H. Nakashima, Y. Kurokawa, and A. Ishikawa, Phys. Rev. Lett. **99**, 240402 (2007).

[4] H. Nakashima and H. Nakatsuji, TSUBAME e-Science J. **11**, 24 (2014).

[5] C. Schwartz, Int. J. Mod. Phys. E **28**, 1 (2006).

[6] C. Wang, Phys. Rev. A **88**, 032511 (2013).

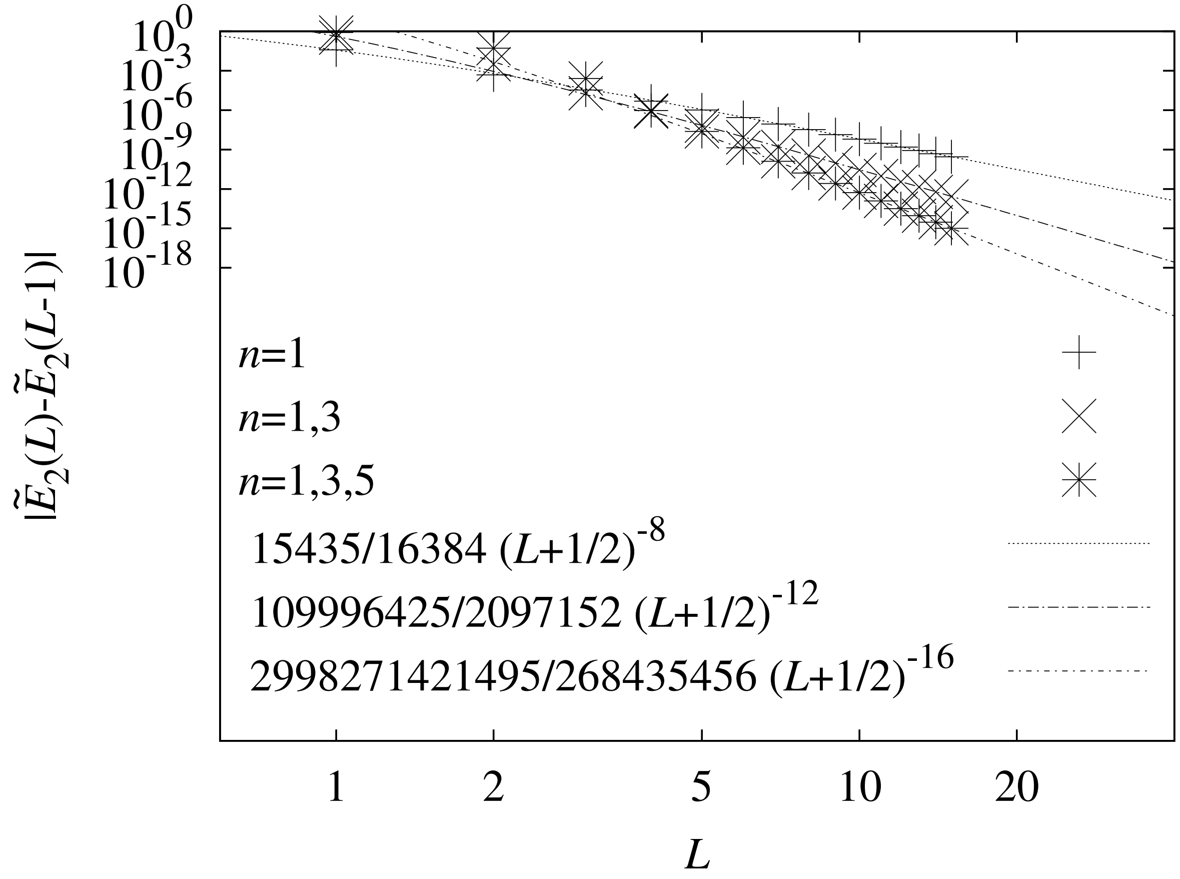


FIG. 3. $|\tilde{E}_2(L)-\tilde{E}_2(L-1)|$ via $L$ plot for the second-order $1/Z$ energy under minimum construction of geminal functions. The numerical data points are obtained from Table III. Atomic units are used in the figure.


[7] C. Schwartz, arXiv:math-ph/0605018 (2006).

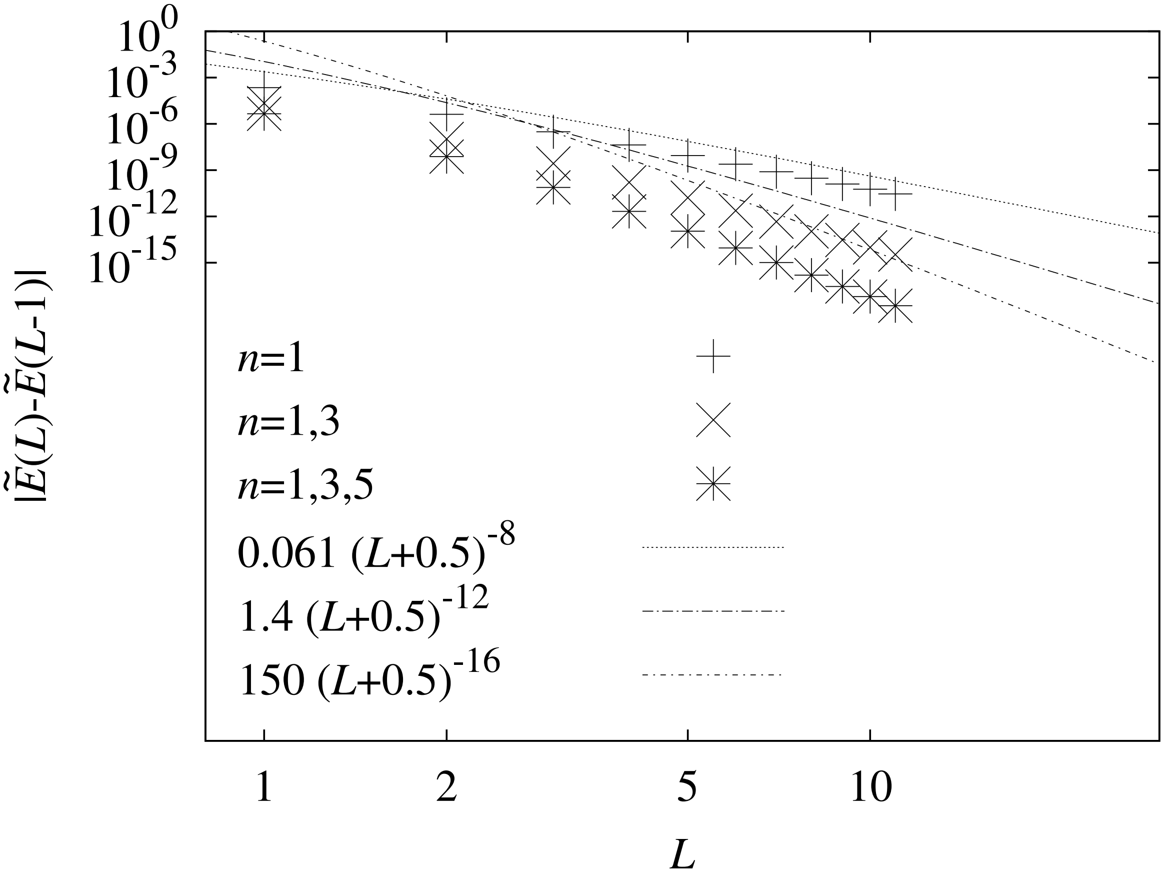


FIG. 4. $|\tilde{E}(L) - \tilde{E}(L-1)|$ via $L$ plot for the Ritz's variational energy. The data of PWE is plotted from Table IV. Atomic units are used in the figure.

TABLE III. Numerical results of the variational PWE increments for the second-order-$1/Z$ expansion energies of the ground state of the helium atom under minimum construction. Eqs. (7) - (9) are used as the wavefunction in the Hylleraas functional [5] at $\omega = 30$. The atomic units are adopted.

| $L$ | $\lvert\tilde{E}_2(L) - \tilde{E}_2(L-1)\rvert$ | | |
|---|---|---|---|
| | $r_{12}\Phi_1 + \tilde{\chi}$ | $r_{12}\Phi_1 + r_{12}^3\Phi_3 + \tilde{\chi}$ | $r_{12}\Phi_1 + r_{12}^3\Phi_3 + r_{12}^5\Phi_5 + \tilde{\chi}$ |
| $0^a$ | $1.179\times10^{-1}$ | $1.721\times10^{-1b}$ | $7.003\times10^{-1b}$ |
| 1 | $3.921\times10^{-2}$ | $3.267\times10^{-1}$ | $8.058\times10^{-1}$ |
| 2 | $4.821\times10^{-4}$ | $3.122\times10^{-3}$ | $5.184\times10^{-2}$ |
| 3 | $3.444\times10^{-5}$ | $1.941\times10^{-5}$ | $2.557\times10^{-4}$ |
| 4 | $4.858\times10^{-6}$ | $7.808\times10^{-7}$ | $9.344\times10^{-7}$ |
| 5 | $1.012\times10^{-7}$ | $6.663\times10^{-8}$ | $2.389\times10^{-8}$ |
| 6 | $2.726\times10^{-7}$ | $8.854\times10^{-9}$ | $1.365\times10^{-10}$ |
| 7 | $8.830\times10^{-8}$ | $1.588\times10^{-10}$ | $1.261\times10^{-11}$ |
| 8 | $3.285\times10^{-8}$ | $3.546\times10^{-10}$ | $1.621\times10^{-12}$ |
| 9 | $1.362\times10^{-9}$ | $9.370\times10^{-11}$ | $2.659\times10^{-12}$ |
| 10 | $6.155\times10^{-9}$ | $2.830\times10^{-11}$ | $5.272\times10^{-13}$ |
| 11 | $2.989\times10^{-9}$ | $9.535\times10^{-12}$ | $1.217\times10^{-14}$ |
| 12 | $1.540\times10^{-10}$ | $3.516\times10^{-12}$ | $3.184\times10^{-14}$ |
| 13 | $8.348\times10^{-10}$ | $1.400\times10^{-13}$ | $9.252\times10^{-15}$ |
| 14 | $4.726\times10^{-10}$ | $5.952\times10^{-13}$ | $2.940\times10^{-15}$ |
| 15 | $2.778\times10^{-10}$ | $2.678\times10^{-13}$ | $1.009\times10^{-15}$ |
| $\Delta E^c$ | $4.210\times10^{-10}$ | $2.066\times10^{-13}$ | $4.331\times10^{-16}$ |

[a] The energy of $\lvert\tilde{E}_2(L)\rvert$, $L$=0.

[b] The energy is positive.

[c] The total energy at the largest $L$ subtracts the reference value, -0.15766 64294 69150 94105 66 a.u. [6]

TABLE IV. Numerical results of the PWE increments for the Ritz variational energies of the ground state helium atom. Basis F at $\omega = 20$ is used . The atomic units are adopted.

| $L$ | $\lvert\tilde{E}(L) - \tilde{E}(L-1)\rvert$ | | |
|---|---|---|---|
| | $\tilde{\Phi}_0 + r_{12}\tilde{\Phi}_1 + \tilde{\chi}$ | $\tilde{\Phi}_0 + r_{12}\tilde{\Phi}_1 + r_{12}^3\tilde{\Phi}_3 + \tilde{\chi}$ | $\tilde{\Phi}_0 + r_{12}\tilde{\Phi}_1 + r_{12}^3\tilde{\Phi}_3 + r_{12}^5\tilde{\Phi}_5 + \tilde{\chi}$ |
| $0^a$ | 2.903 | 2.904 | 2.904 |
| 1 | $2.216\times10^{-4}$ | $2.200\times10^{-5}$ | $4.488\times10^{-6}$ |
| 2 | $4.121\times10^{-6}$ | $1.057\times10^{-7}$ | $7.457\times10^{-9}$ |
| 3 | $3.033\times10^{-7}$ | $2.680\times10^{-9}$ | $7.639\times10^{-11}$ |
| 4 | $4.268\times10^{-8}$ | $1.592\times10^{-10}$ | $2.096\times10^{-12}$ |
| 5 | $8.864\times10^{-9}$ | $1.613\times10^{-11}$ | $1.093\times10^{-13}$ |
| 6 | $2.398\times10^{-9}$ | $2.365\times10^{-12}$ | $8.984\times10^{-15}$ |
| 7 | $7.831\times10^{-10}$ | $4.533\times10^{-13}$ | $1.033\times10^{-15}$ |
| 8 | $2.952\times10^{-10}$ | $1.076\times10^{-13}$ | $1.561\times10^{-16}$ |
| 9 | $1.253\times10^{-10}$ | $2.972\times10^{-14}$ | $2.871\times10^{-17}$ |
| 10 | $5.811\times10^{-11}$ | $9.643\times10^{-15}$ | $6.405\times10^{-18}$ |
| 11 | $2.878\times10^{-11}$ | $3.345\times10^{-15}$ | $1.613\times10^{-18}$ |
| $\Delta E^b$ | $4.304\times10^{-11}$ | $2.493\times10^{-15}$ | $7.239\times10^{-19}$ |

[a] The energy of $\lvert\tilde{E}(L)\rvert$, $L$=0.

[b] Total energy at the largest $L$ subtracts the reference value - 2.903 724 377 034 119 598 311 [7].

TABLE V. Numerical results of the PWE increments for the non-perturbative ground state of the helium atom by expanding the reference wavefunction under the minimum construction of geminal functions. Basis F at $\omega = 14$ is used for the reference wavefunction. The atomic units are adopted.

| $L$ | $\|E(L) - E(L-1)\|$ | | |
|---|---|---|---|
| | $\Phi_0 + r_{12}\Phi_1 + \chi$ | $\Phi_0 + r_{12}\Phi_1 + r_{12}^3\Phi_3 + \chi$ | $\Phi_0 + r_{12}\Phi_1 + r_{12}^3\Phi_3 + r_{12}^5\Phi_5 + \chi$ |
| $0^a$ | 2.895 | 2.807 | 2.832 |
| 1 | $9.038\times10^{-3}$ | $4.045\times10^{-2}$ | $6.904\times10^{-2}$ |
| 2 | $8.210\times10^{-5}$ | $2.620\times10^{-4}$ | $2.783\times10^{-3}$ |
| 3 | $5.265\times10^{-6}$ | $1.418\times10^{-7}$ | $1.130\times10^{-6}$ |
| 4 | $7.028\times10^{-7}$ | $5.330\times10^{-8}$ | $3.741\times10^{-8}$ |
| 5 | $1.416\times10^{-8}$ | $4.372\times10^{-9}$ | $9.024\times10^{-10}$ |
| 6 | $3.733\times10^{-8}$ | $5.661\times10^{-10}$ | $4.965\times10^{-11}$ |
| 7 | $1.191\times10^{-9}$ | $9.975\times10^{-11}$ | $4.468\times10^{-12}$ |
| 8 | $4.383\times10^{-9}$ | $2.199\times10^{-11}$ | $5.631\times10^{-13}$ |
| 9 | $1.802\times10^{-10}$ | $5.760\times10^{-12}$ | $9.100\times10^{-14}$ |
| 10 | $8.096\times10^{-10}$ | $1.726\times10^{-12}$ | $1.780\times10^{-15}$ |
| 11 | $3.912\times10^{-10}$ | $5.779\times10^{-13}$ | $4.077\times10^{-15}$ |
| $\Delta E^b$ | $4.695\times10^{-10}$ | $3.637\times10^{-13}$ | $1.663\ \times10^{-15}$ |

$^a$ The energy of $|E(L)|$, $L$=0.

$^b$ Total energy at the largest $L$ subtracts the reference value - 2.903 724 377 034 119 598 311 [7].

TABLE VI. Numerical results of the PWE increments for the Ritz variational energies of the ground state helium atom under the minimum construction of geminal functions. Basis F at $\omega = 20$ is use. The atomic units are adopted.

| $L$ | $\lvert\tilde{E}(L) - \tilde{E}(L-1)\rvert$ | | |
|---|---|---|---|
| | $\tilde{\Phi}_0 + r_{12}\tilde{\Phi}_1 + \tilde{\chi}$ | $\tilde{\Phi}_0 + r_{12}\tilde{\Phi}_1 + r_{12}^3\tilde{\Phi}_3 + \tilde{\chi}$ | $\tilde{\Phi}_0 + r_{12}\tilde{\Phi}_1 + r_{12}^3\tilde{\Phi}_3 + r_{12}^5\tilde{\Phi}_5 + \tilde{\chi}$ |
| 0[a] | 2.903 | 2.904 | 2.904 |
| 1 | $6.014\times10^{-4}$ | $5.397\times10^{-5}$ | $1.013\times10^{-5}$ |
| 2 | $1.754\times10^{-5}$ | $4.509\times10^{-7}$ | $2.758\times10^{-8}$ |
| 3 | $1.549\times10^{-6}$ | $1.628\times10^{-8}$ | $4.228\times10^{-10}$ |
| 4 | $2.378\times10^{-7}$ | $1.235\times10^{-9}$ | $1.673\times10^{-11}$ |
| 5 | $5.184\times10^{-8}$ | $1.522\times10^{-10}$ | $1.297\times10^{-12}$ |
| 6 | $1.449\times10^{-8}$ | $2.788\times10^{-11}$ | $1.827\times10^{-13}$ |
| 7 | $4.914\times10^{-9}$ | $7.150\times10^{-12}$ | $2.969\times10^{-14}$ |
| 8 | $1.966\times10^{-9}$ | $2.185\times10^{-12}$ | $4.876\times10^{-15}$ |
| 9 | $9.131\times10^{-10}$ | $6.931\times10^{-13}$ | $1.050\times10^{-15}$ |
| 10 | $4.848\times10^{-10}$ | $2.264\times10^{-13}$ | $4.167\times10^{-16}$ |
| 11 | $2.881\times10^{-10}$ | $7.891\times10^{-14}$ | $2.620\times10^{-16}$ |
| $\Delta E$[b] | $1.000\times10^{-9}$ | $1.321\times10^{-13}$ | $4.083\times10^{-16}$ |

[a] The energy of $\lvert\tilde{E}(L)\rvert$, $L$=0.

[b] Total energy at the largest $L$ subtracts the reference value - 2.903 724 377 034 119 598 311 [7].

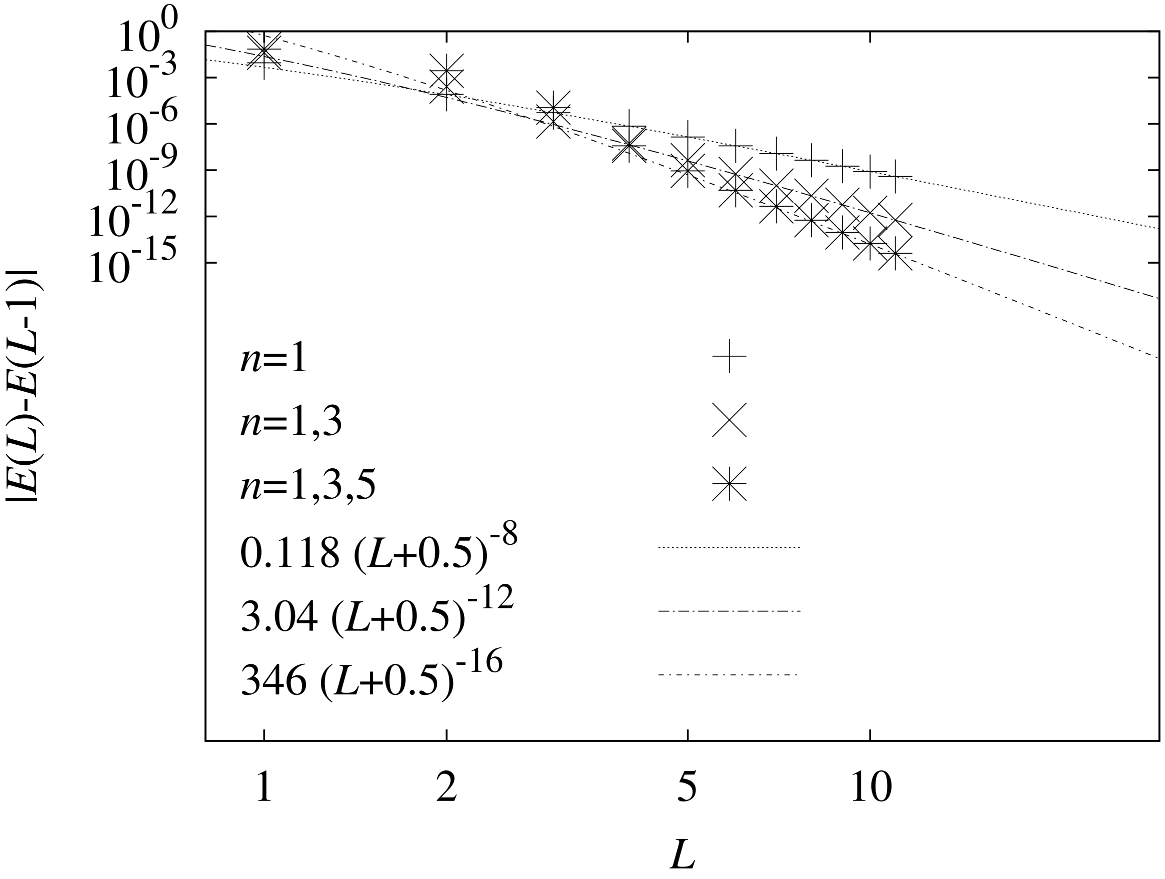


FIG. 5. $|E(L) - E(L-1)|$ via $L$ plot for the PWE from the reference wavefunction under minimum construction of geminal functions. The data of PWE is plotted from Table V. Atomic units are used in the figure.

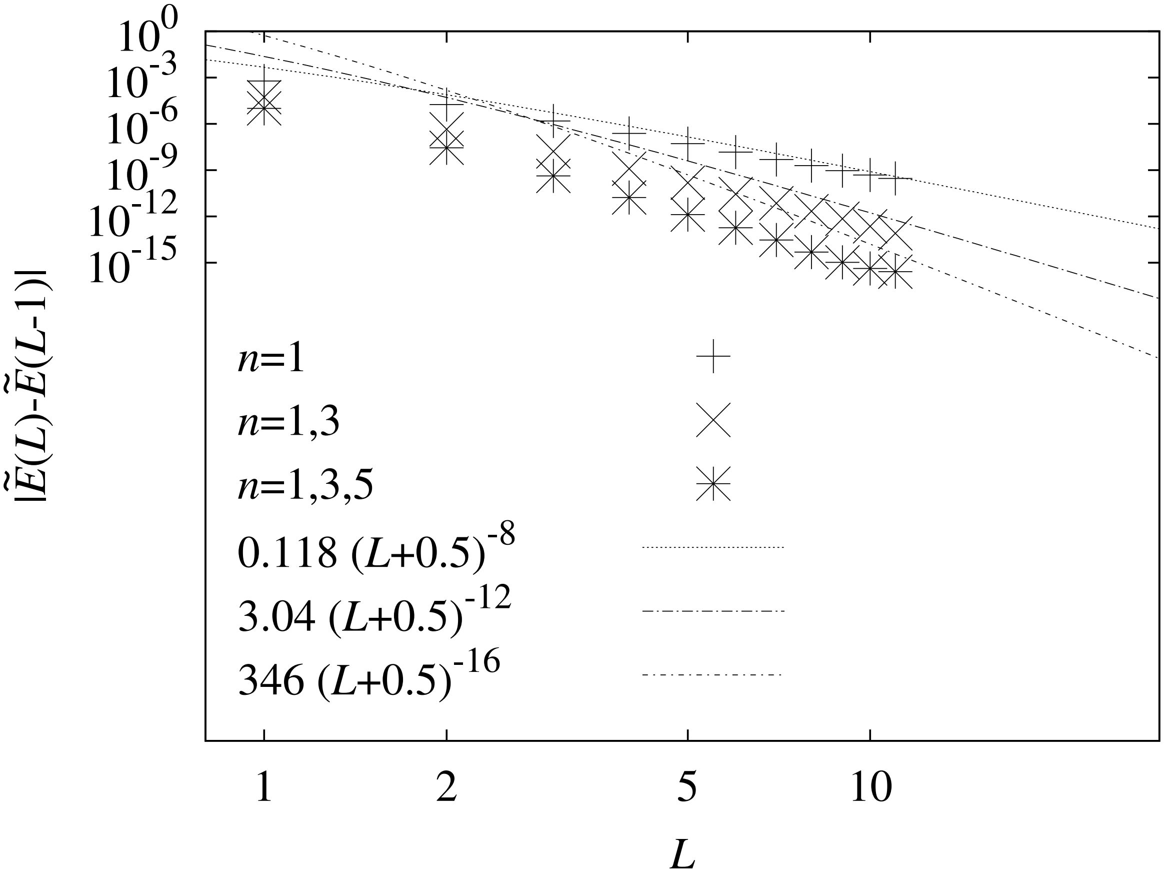


FIG. 6. $|\tilde{E}(L)-\tilde{E}(L-1)|$ via $L$ plot for the Ritz's variational energy under minimum construction of geminal functions. The data of PWE is plotted from Table VI. Atomic units are used in the figure.

TABLE VII. Numerical results of the expanded PWE energies for the second-order-$1/Z$ expansion energies of the ground state of the helium atom. Basis F [5] with $\omega = 20$ is used. The atomic units are adopted.

| $L$ | $E_2(L)$ | | |
|---|---|---|---|
| | $\Phi_0 + r_{12}\Phi_1 + \chi$ | $\Phi_0 + r_{12}\Phi_1 + r_{12}^3\Phi_3 + \chi$ | $\Phi_0 + r_{12}\Phi_1 + r_{12}^3\Phi_3 + r_{12}^5\Phi_5 + \chi$ |
| 0 | -0.12827 44228 26619 50899 | 0.10306 57335 72523 50069 | 0.57224 54742 15785 02286 |
| 1 | -0.15730 95254 81033 98651 | -0.15551 28486 10326 06580 | -0.11848 95026 57901 82771 |
| 2 | -0.15763 94894 62355 95549 | -0.15765 37136 66926 68151 | -0.15749 40014 19157 79988 |
| 3 | -0.15766 23307 89744 89543 | -0.15766 59197 66645 89241 | -0.15766 58396 18027 48877 |
| 4 | -0.15766 55040 03670 44288 | -0.15766 63850 02802 29882 | -0.15766 64148 72272 93291 |
| 5 | -0.15766 61592 56752 54238 | -0.15766 64233 46853 12298 | -0.15766 64286 43447 07433 |
| 6 | -0.15766 63348 81039 25712 | -0.15766 64283 23231 04618 | -0.15766 64293 92453 51208 |
| 7 | -0.15766 63915 71530 76249 | -0.15766 64292 01132 84533 | -0.15766 64294 59140 87900 |
| 8 | -0.15766 64126 13545 84694 | -0.15766 64293 94864 00698 | -0.15766 64294 67471 98666 |
| 9 | -0.15766 64213 22163 66559 | -0.15766 64294 45609 18183 | -0.15766 64294 68809 07258 |
| 10 | -0.15766 64252 55222 96113 | -0.15766 64294 60835 39874 | -0.15766 64294 69069 66307 |
| 11 | -0.15766 64271 63340 24476 | -0.15766 64294 65937 91495 | -0.15766 64294 69129 00235 |
| 12 | -0.15766 64281 46084 52840 | -0.15766 64294 67812 14350 | -0.15766 64294 69144 35698 |
| 13 | -0.15766 64286 78534 82207 | -0.15766 64294 68556 00407 | -0.15766 64294 69148 77904 |
| 14 | -0.15766 64288 73898 38321 | -0.15766 64294 68871 45879 | -0.15766 64294 69150 17398 |
| 15 | -0.15766 64289 79838 10244 | -0.15766 64294 69013 13330 | -0.15766 64294 69150 64992 |

TABLE VIII. Numerical results of the variational PWE energies for the second-order-$1/Z$ expansion energies of the ground state of the helium atom. Basis F [5] with $\omega = 30$ is used. The atomic units are adopted.

| $L$ | $\tilde{E}_2(L)$ | | |
|---|---|---|---|
| | $r_{12}\Phi_1 + \tilde{\chi}$ | $r_{12}\Phi_1 + r_{12}^3\Phi_3 + \tilde{\chi}$ | $r_{12}\Phi_1 + r_{12}^3\Phi_3 + r_{12}^5\Phi_5 + \tilde{\chi}$ |
| 0 | -0.12823 20686 92610 31632 | 0.11413 53625 44021 64353 | 0.60889 05783 09089 22554 |
| 1 | -0.15730 95591 94762 11997 | -0.15546 52368 47495 53371 | -0.11740 28121 72674 61250 |
| 2 | -0.15763 94928 61483 87409 | -0.15765 35761 44953 28718 | -0.15749 28585 91211 76343 |
| 3 | -0.15766 23310 41027 82299 | -0.15766 59168 69568 78163 | -0.15766 58440 74109 27871 |
| 4 | -0.15766 55040 01925 00186 | -0.15766 63848 58892 78723 | -0.15766 64150 97562 98817 |
| 5 | -0.15766 61592 18893 53966 | -0.15766 64233 34767 78949 | -0.15766 64286 59150 97075 |
| 6 | -0.15766 63348 29094 47667 | -0.15766 64283 21742 03595 | -0.15766 64293 93990 49159 |
| 7 | -0.15766 63915 08940 26776 | -0.15766 64292 00856 71025 | -0.15766 64294 59337 59206 |
| 8 | -0.15766 64125 41640 93534 | -0.15766 64293 94765 25675 | -0.15766 64294 67503 07110 |
| 9 | -0.15766 64212 42063 69638 | -0.15766 64294 45539 97076 | -0.15766 64294 68814 82784 |
| 10 | -0.15766 64251 68029 92828 | -0.15766 64294 60770 44491 | -0.15766 64294 69070 80974 |
| 11 | -0.15766 64270 70111 95855 | -0.15766 64294 65872 55143 | -0.15766 64294 69129 17960 |
| 12 | -0.15766 64280 47794 16254 | -0.15766 64294 67745 67968 | -0.15766 64294 69144 30332 |
| 13 | -0.15766 64285 76046 47722 | -0.15766 64294 68488 54744 | -0.15766 64294 69148 66096 |
| 14 | -0.15766 64288 73898 38321 | -0.15766 64294 68803 23912 | -0.15766 64294 69150 03785 |
| 15 | -0.15766 64290 48137 20035 | -0.15766 64294 68944 35657 | -0.15766 64294 69150 50795 |

TABLE IX. Numerical results of the expanded PWE energies for the second-order-$1/Z$ expansion energies of the ground state of the helium atom under minimum construction. Basis F [5] with $\omega = 20$ is used. The atomic units are adopted.

| $L$ | $E_2(L)$ | | |
|---|---|---|---|
| | $r_{12}\Phi_1 + \chi$ | $r_{12}\Phi_1 + r_{12}^3\Phi_3 + \chi$ | $r_{12}\Phi_1 + r_{12}^3\Phi_3 + r_{12}^5\Phi_5 + \chi$ |
| 0 | -0.11793 12618 77135 82403 | 0.17214 41549 86088 39159 | 0.70006 70635 66720 17617 |
| 1 | -0.15714 35989 07465 21280 | -0.15452 43199 20764 46586 | -0.10559 39777 21694 91531 |
| 2 | -0.15762 57013 57354 11578 | -0.15764 61586 00359 31104 | -0.15740 99755 00878 40061 |
| 3 | -0.15766 01388 68710 77096 | -0.15766 55710 72494 15837 | -0.15766 54705 26561 57966 |
| 4 | -0.15766 49973 55623 94258 | -0.15766 63518 98470 83603 | -0.15766 64040 97430 22635 |
| 5 | -0.15766 60092 70465 70719 | -0.15766 64185 35019 26680 | -0.15766 64279 60951 06762 |
| 6 | -0.15766 62819 15145 98187 | -0.15766 64273 89043 29053 | -0.15766 64293 23787 66175 |
| 7 | -0.15766 63702 24595 29730 | -0.15766 64289 76947 14820 | -0.15766 64294 49645 09191 |
| 8 | -0.15766 64030 79669 07472 | -0.15766 64293 31554 19082 | -0.15766 64294 65809 57131 |
| 9 | -0.15766 64167 00119 80720 | -0.15766 64294 25263 85873 | -0.15766 64294 68459 47611 |
| 10 | -0.15766 64228 59107 61552 | -0.15766 64294 53571 62529 | -0.15766 64294 68984 47957 |
| 11 | -0.15766 64258 49931 25128 | -0.15766 64294 63107 70926 | -0.15766 64294 69105 57154 |
| 12 | -0.15766 64273 91425 48377 | -0.15766 64294 66624 98285 | -0.15766 64294 69137 22241 |
| 13 | -0.15766 64282 27086 40764 | -0.15766 64294 68025 60456 | -0.15766 64294 69146 41021 |
| 14 | -0.15766 64287 00189 35761 | -0.15766 64294 68621 19197 | -0.15766 64294 69149 32657 |
| 15 | -0.15766 64289 78309 15452 | -0.15766 64294 68889 27804 | -0.15766 64294 69150 32643 |

TABLE X. Numerical results of the variational PWE energies for the second-order-$1/Z$ expansion energies of the ground state of the helium atom under minimum construction. Basis F [5] with $\omega = 30$ is used. The atomic units are adopted.

| $L$ | $\tilde{E}_2(L)$ | | |
|---|---|---|---|
| | $r_{12}\Phi_1 + \tilde{\chi}$ | $r_{12}\Phi_1 + r_{12}^3\Phi_3 + \tilde{\chi}$ | $r_{12}\Phi_1 + r_{12}^3\Phi_3 + r_{12}^5\Phi_5 + \tilde{\chi}$ |
| 0 | -0.11793 12617 54312 70424 | 0.17214 26674 33086 54259 | 0.70027 55334 53824 41461 |
| 1 | -0.15714 35988 92862 88010 | -0.15452 43453 44603 24318 | -0.10557 29559 35468 44837 |
| 2 | -0.15762 57013 32972 53615 | -0.15764 61588 55006 82913 | -0.15740 98172 75396 58864 |
| 3 | -0.15766 01388 29616 53518 | -0.15766 55710 88094 39073 | -0.15766 54696 63897 76525 |
| 4 | -0.15766 49973 01035 08164 | -0.15766 63519 00411 13079 | -0.15766 64040 65541 49760 |
| 5 | -0.15766 60092 01394 95248 | -0.15766 64185 35378 85042 | -0.15766 64279 58395 97847 |
| 6 | -0.15766 62818 33662 09888 | -0.15766 64273 89127 62304 | -0.15766 64293 23465 18653 |
| 7 | -0.15766 63701 33207 28016 | -0.15766 64289 76968 16388 | -0.15766 64294 49589 72823 |
| 8 | -0.15766 64029 80852 64769 | -0.15766 64293 31557 01141 | -0.15766 64294 65797 66068 |
| 9 | -0.15766 64165 96027 43855 | -0.15766 64294 25260 19146 | -0.15766 64294 68456 42493 |
| 10 | -0.15766 64227 51446 28700 | -0.15766 64294 53565 06672 | -0.15766 64294 68983 57893 |
| 11 | -0.15766 64257 39959 15430 | -0.15766 64294 63099 58738 | -0.15766 64294 69105 27106 |
| 12 | -0.15766 64272 80014 25832 | -0.15766 64294 66615 90512 | -0.15766 64294 69137 10970 |
| 13 | -0.15766 64281 14807 22425 | -0.15766 64294 68015 90943 | -0.15766 64294 69146 36213 |
| 14 | -0.15766 64285 87397 14536 | -0.15766 64294 68611 09290 | -0.15766 64294 69149 30259 |
| 15 | -0.15766 64288 65212 80579 | -0.15766 64294 68878 91659 | -0.15766 64294 69150 31207 |

TABLE XI. Numerical results of the PWE energies for the non-perturbative ground state helium atom by expanding the reference wavefunction. Basis F at $\omega = 14$ is used for the reference wavefunction. The atomic units are adopted.

| $L$ | $E(L)$ | | |
|---|---|---|---|
| | $\Phi_0 + r_{12}\Phi_1 + \chi$ | $\Phi_0 + r_{12}\Phi_1 + r_{12}^3\Phi_3 + \chi$ | $\Phi_0 + r_{12}\Phi_1 + r_{12}^3\Phi_3 + r_{12}^5\Phi_5 + \chi$ |
| 0 | -2.89704 63882 35423 27463 | -2.86301 01549 08175 15774 | -2.83188 83112 06827 92527 |
| 1 | -2.90367 04456 83005 55805 | -2.90346 09181 29380 68473 | -2.90092 96243 69107 65598 |
| 2 | -2.90372 08820 89198 27219 | -2.90372 29007 21645 89211 | -2.90371 30366 92076 26416 |
| 3 | -2.90372 38842 55510 81016 | -2.90372 43186 70813 82350 | -2.90372 43386 64731 29450 |
| 4 | -2.90372 42705 34273 74635 | -2.90372 43719 66274 51905 | -2.90372 43760 76893 54470 |
| 5 | -2.90372 43467 86706 78799 | -2.90372 43763 37828 36759 | -2.90372 43769 79328 32972 |
| 6 | -2.90372 43666 41539 26963 | -2.90372 43769 03961 16827 | -2.90372 43770 28974 00178 |
| 7 | -2.90372 43729 24917 13561 | -2.90372 43770 03706 64985 | -2.90372 43770 33441 86110 |
| 8 | -2.90372 43752 24222 00128 | -2.90372 43770 25696 94545 | -2.90372 43770 34005 00989 |
| 9 | -2.90372 43761 65800 29844 | -2.90372 43770 31452 33315 | -2.90372 43770 34096 02578 |
| 10 | -2.90372 43765 87595 43983 | -2.90372 43770 33178 00234 | -2.90372 43770 34113 85885 |
| 11 | -2.90372 43767 90920 20913 | -2.90372 43770 33755 91488 | -2.90372 43770 34117 93570 |

TABLE XII. Numerical results of the PWE increments for the Ritz variational energies of the ground state helium atom. Basis F at $\omega = 20$ is used . The atomic units are adopted.

| $L$ | $\tilde{E}(L)$ | | |
|---|---|---|---|
| | $\tilde{\Phi}_0 + r_{12}\tilde{\Phi}_1 + \tilde{\chi}$ | $\tilde{\Phi}_0 + r_{12}\tilde{\Phi}_1 + r_{12}^3\tilde{\Phi}_3 + \tilde{\chi}$ | $\tilde{\Phi}_0 + r_{12}\tilde{\Phi}_1 + r_{12}^3\tilde{\Phi}_3 + r_{12}^5\tilde{\Phi}_5 + \tilde{\chi}$ |
| 0 | -2.90349 82755 29045 02041 | -2.90370 22655 39866 01672 | -2.90370 22655 39866 01672 |
| 1 | -2.90371 98977 97159 43590 | -2.90372 42685 13951 00804 | -2.90372 42685 13951 00804 |
| 2 | -2.90372 40184 50318 94169 | -2.90372 43741 76294 83428 | -2.90372 43741 76294 83428 |
| 3 | -2.90372 43217 55650 40449 | -2.90372 43768 55818 64111 | -2.90372 43768 55818 64111 |
| 4 | -2.90372 43644 38352 15831 | -2.90372 43770 15021 89890 | -2.90371 98816 46196 83167 |
| 5 | -2.90372 43733 02152 74764 | -2.90372 43770 31148 94272 | -2.90372 43694 98596 97349 |
| 6 | -2.90372 43757 00619 98551 | -2.90372 43770 33513 52434 | -2.90372 43769 55518 29866 |
| 7 | -2.90372 43764 83722 12467 | -2.90372 43770 33966 83493 | -2.90372 43770 31903 69481 |
| 8 | -2.90372 43767 78898 80710 | -2.90372 43770 34074 39553 | -2.90372 43770 34000 05222 |
| 9 | -2.90372 43769 04187 35664 | -2.90372 43770 34104 11721 | -2.90372 43770 34109 38770 |
| 10 | -2.90372 43769 62300 68416 | -2.90372 43770 34113 76069 | -2.90372 43770 34118 37193 |
| 11 | -2.90372 43769 91079 18868 | -2.90372 43770 34117 10574 | -2.90372 43770 34119 40476 |

TABLE XIII. Numerical results of the PWE increments for the non-perturbative ground state of the helium atom by expanding the reference wavefunction under the minimum construction of geminal functions. Basis F at $\omega = 14$ is used for the reference wavefunction. The atomic units are adopted.

| $L$ | $E(L)$ | | |
|---|---|---|---|
| | $\Phi_0 + r_{12}\Phi_1 + \chi$ | $\Phi_0 + r_{12}\Phi_1 + r_{12}^3\Phi_3 + \chi$ | $\Phi_0 + r_{12}\Phi_1 + r_{12}^3\Phi_3 + r_{12}^5\Phi_5 + \chi$ |
| 0 | -2.89459 82266 11717 08713 | -2.86301 01549 08175 15774 | -2.86301 01549 08175 15774 |
| 1 | -2.90363 61081 13351 61921 | -2.90346 09181 29380 68473 | -2.90346 09181 29380 68473 |
| 2 | -2.90371 82104 81357 66667 | -2.90372 29007 21645 89211 | -2.90372 29007 21645 89211 |
| 3 | -2.90372 34755 56878 79161 | -2.90372 43186 70813 82350 | -2.90372 43186 70813 82350 |
| 4 | -2.90372 41783 42586 44321 | -2.90372 43719 66274 51905 | -2.90372 43719 66274 51905 |
| 5 | -2.90372 43199 38062 48808 | -2.90372 43763 37828 36759 | -2.90372 43763 37828 36759 |
| 6 | -2.90372 43572 68773 62329 | -2.90372 43769 03961 16827 | -2.90372 43769 03961 16827 |
| 7 | -2.90372 43691 78987 39157 | -2.90372 43770 03706 64985 | -2.90372 43770 03706 64985 |
| 8 | -2.90372 43735 61776 96392 | -2.90372 43770 25696 94545 | -2.90372 43770 25696 94545 |
| 9 | -2.90372 43753 63775 27073 | -2.90372 43770 31452 33315 | -2.90372 43770 31452 33315 |
| 10 | -2.90372 43761 73423 00923 | -2.90372 43770 33178 00234 | -2.90372 43770 33178 00234 |
| 11 | -2.90372 43765 64602 93540 | -2.90372 43770 33755 91488 | -2.90372 43770 33755 91488 |

TABLE XIV. Numerical results of the PWE increments for the Ritz variational energies of the ground state helium atom. Basis F at $\omega = 20$ is used under minimum construction. The atomic units are adopted.

| $L$ | $\tilde{E}(L)$ | | |
|---|---|---|---|
| | $\tilde{\Phi}_0 + r_{12}\tilde{\Phi}_1 + \tilde{\chi}$ | $\tilde{\Phi}_0 + r_{12}\tilde{\Phi}_1 + r_{12}^3\tilde{\Phi}_3 + \tilde{\chi}$ | $\tilde{\Phi}_0 + r_{12}\tilde{\Phi}_1 + r_{12}^3\tilde{\Phi}_3 + r_{12}^5\tilde{\Phi}_5 + \tilde{\chi}$ |
| 0 | -2.90310 35841 40745 65722 | -2.90366 99335 63533 31131 | -2.90371 42236 98644 18006 |
| 1 | -2.90370 49741 28616 93420 | -2.90372 39083 96886 45715 | -2.90372 43490 12745 20160 |
| 2 | -2.90372 25147 30638 05298 | -2.90372 43593 25103 05664 | -2.90372 43765 93021 72302 |
| 3 | -2.90372 40633 20390 94298 | -2.90372 43756 08985 95412 | -2.90372 43770 15868 24630 |
| 4 | -2.90372 43011 36573 40094 | -2.90372 43768 43545 68472 | -2.90372 43770 32602 96927 |
| 5 | -2.90372 43529 79285 59283 | -2.90372 43769 95777 74396 | -2.90372 43770 33900 16175 |
| 6 | -2.90372 43674 67368 16989 | -2.90372 43770 23654 29392 | -2.90372 43770 34082 89974 |
| 7 | -2.90372 43723 81640 36938 | -2.90372 43770 30804 11744 | -2.90372 43770 34112 58490 |
| 8 | -2.90372 43743 47844 87502 | -2.90372 43770 32989 14092 | -2.90372 43770 34117 46094 |
| 9 | -2.90372 43752 60994 31529 | -2.90372 43770 33682 19308 | -2.90372 43770 34118 51131 |
| 10 | -2.90372 43757 45822 66363 | -2.90372 43770 33908 62468 | -2.90372 43770 34118 92798 |
| 11 | -2.90372 43760 33923 31119 | -2.90372 43770 33987 53081 | -2.90372 43770 34119 19001 |
